# Supplementary material for: Minimally Supervised Topological Projections of Self-Organizing Maps for Phase of Flight Identification
Source: arXiv:2402.11185 source file (2024-02-17)
Supplement: Supplementary file 1 [file 81-appendix.tex]

\newpage

\section{Appendix}

% file 38 validation
\begin{table*}[!t]\centering
\caption{38 Validation 5}\label{tab:38_5_vali }
\scriptsize
\begin{tabular}{c|ccc|ccc|ccc}\toprule
&\multicolumn{3}{c|}{Minmax Norm} &\multicolumn{3}{c|}{Standard Norm} &\multicolumn{3}{c}{Robust Norm} \\\cmidrule{2-10}
&3 &5 &7   &3 &5 &7  &3 &5 &7   \\\midrule
5 x 5 & 26.67 & 16.67 & 16.67 & 50.00 & 36.67 & 13.33 & 23.33 & 20.00 & 6.67 \\ 
7 x 7 & 66.67 & 50.00 & 40.00 & 53.33 & 30.00 & 26.67 & 33.33 & 26.67 & 13.33 \\ 
10 x 10 & \bf{70.00} & 43.33 & 30.00 & 66.67 & 50.00 & 23.33 & 33.33 & 26.67 & 23.33 \\ 

\bottomrule
\end{tabular}
\end{table*}

\begin{table*}[!t]\centering
\caption{38 Validation 10}\label{tab:38_10_vali }
\scriptsize
\begin{tabular}{c|cccc|cccc|cccc}\toprule
&\multicolumn{4}{c|}{Minmax Norm} &\multicolumn{4}{c|}{Standard Norm} &\multicolumn{4}{c}{Robust Norm} \\\cmidrule{2-13}
&3 &5 &7 &10  &3 &5 &7 &10  &3 &5 &7 &10  \\\midrule
5 x 5 & 53.33 & 53.33 & 25.00 & 25.00 & 51.67 & 48.33 & 38.33 & 21.67 & 30.00 & 23.33 & 26.67 & 30.00 \\ 
7 x 7 & 50.00 & 55.00 & 56.67 & 65.00 & 61.67 & 61.67 & 58.33 & 46.67 & 48.33 & 40.00 & 30.00 & 35.00 \\ 
10 x 10 & 70.00 & 70.00 & 65.00 & 60.00 & \bf{81.67} & 76.67 & 76.67 & 53.33 & 38.33 & 31.67 & 38.33 & 30.00 \\ 
15 x 15 & 60.00 & 58.33 & 53.33 & 55.00 & 68.33 & 73.33 & 66.67 & 65.00 & 51.67 & 43.33 & 45.00 & 46.67 \\

\bottomrule
\end{tabular}
\end{table*}

\begin{table*}[!t]\centering
\caption{38 Validation 20}\label{tab:38_10_vali }
\scriptsize
\begin{tabular}{c|ccccc|ccccc|ccccc}\toprule
&\multicolumn{5}{c|}{Minmax Norm} &\multicolumn{5}{c|}{Standard Norm} &\multicolumn{5}{c}{Robust Norm} \\\cmidrule{2-16}
&3 &5 &7 &10 &15 &3 &5 &7 &10 &15 &3 &5 &7 &10 &15 \\\midrule
5 x 5 & 62.07 & 56.90 & 58.62 & 59.48 & 29.31 & 51.72 & 56.03 & 51.72 & 50.86 & 52.59 & 47.41 & 44.83 & 40.52 & 41.38 & 30.17 \\ 
7 x 7 & 60.34 & 69.83 & 67.24 & 75.00 & 62.93 & 46.55 & 42.24 & 43.10 & 45.69 & 44.83 & 61.21 & 49.14 & 48.28 & 48.28 & 44.83 \\ 
10 x 10 & 78.45 & 85.34 & 85.34 & 81.03 & 81.90 & 68.10 & 83.62 & 84.48 & 84.48 & 69.83 & 61.21 & 52.59 & 60.34 & 58.62 & 53.45 \\ 
15 x 15 & \bf{91.38} & 87.07 & 84.48 & 82.76 & 65.52 & 82.76 & 83.62 & 81.90 & 83.62 & 81.03 & 77.59 & 75.86 & 63.79 & 61.21 & 57.76 \\ 
20 x 20 & 84.48 & 79.31 & 81.90 & 79.31 & 65.52 & 80.17 & 80.17 & 79.31 & 80.17 & 73.28 & 75.86 & 74.14 & 73.28 & 72.41 & 61.21 \\ 
25 x 25 & 87.93 & 86.21 & 85.34 & 84.48 & 78.45 & 82.76 & 79.31 & 79.31 & 75.00 & 73.28 & 75.86 & 76.72 & 70.69 & 77.59 & 63.79 \\ 
\bottomrule
\end{tabular}
\end{table*}

% file 38 testing
% \begin{table*}[!t]\centering
% \caption{38 testing 5}\label{tab:38_test_38 }
% \scriptsize
% \begin{tabular}{c|ccc|ccc|ccc}\toprule
% &\multicolumn{3}{c|}{Minmax Norm} &\multicolumn{3}{c|}{Standard Norm} &\multicolumn{3}{c}{Robust Norm} \\\cmidrule{2-10}
% &3 &5 &7   &3 &5 &7  &3 &5 &7   \\\midrule

% \bottomrule
% \end{tabular}
% \end{table*}

% \begin{table*}[!t]\centering
% \caption{38 testing 10}\label{tab:38_test_38 }
% \scriptsize
% \begin{tabular}{c|cccc|cccc|cccc}\toprule
% &\multicolumn{4}{c|}{Minmax Norm} &\multicolumn{4}{c|}{Standard Norm} &\multicolumn{4}{c}{Robust Norm} \\\cmidrule{2-13}
% &3 &5 &7 &10  &3 &5 &7 &10  &3 &5 &7 &10  \\\midrule

% \bottomrule
% \end{tabular}
% \end{table*}
\begin{table*}[!t]\centering
\caption{38 Testing 38 5}\label{tab:38_test }
\scriptsize
\begin{tabular}{c|ccc|ccc|ccc}\toprule
&\multicolumn{3}{c|}{Minmax Norm} &\multicolumn{3}{c|}{Standard Norm} &\multicolumn{3}{c}{Robust Norm} \\\cmidrule{2-10}
&3 &5 &7   &3 &5 &7  &3 &5 &7   \\\midrule
5 x 5 & 37.08 & 27.88 & 18.83 & 56.28 & 48.96 & 19.49 & 37.87 & 40.52 & 24.97 \\ 
7 x 7 & 70.46 & 51.12 & 48.06 & 62.02 & 62.76 & 60.78 & 47.08 & 42.74 & 24.33 \\ 
10 x 10 & \bf{78.60} & 58.19 & 41.44 & 78.34 & 64.69 & 40.44 & 45.83 & 34.83 & 45.83 \\ 

\bottomrule
\end{tabular}
\end{table*}

\begin{table*}[!t]\centering
\caption{38 testing 38 10}\label{tab:343638_vali }
\scriptsize
\begin{tabular}{c|cccc|cccc|cccc}\toprule
&\multicolumn{4}{c|}{Minmax Norm} &\multicolumn{4}{c|}{Standard Norm} &\multicolumn{4}{c}{Robust Norm} \\\cmidrule{2-13}
&3 &5 &7 &10  &3 &5 &7 &10  &3 &5 &7 &10  \\\midrule
5 x 5 & 69.16 & 68.79 & 33.51 & 32.40 & 59.06 & 67.18 & 56.65 & 36.23 & 37.98 & 45.20 & 44.59 & 43.75 \\ 
7 x 7 & 63.87 & 67.18 & 69.69 & 69.32 & 71.36 & 65.01 & 64.61 & 59.93 & 41.92 & 43.19 & 28.72 & 39.57 \\ 
10 x 10 & 80.69 & \bf{82.12} & 76.17 & 67.36 & 78.47 & 79.53 & 78.26 & 59.16 & 53.82 & 47.39 & 51.89 & 44.27 \\ 
15 x 15 & 76.36 & 73.84 & 72.68 & 59.77 & 74.66 & 76.17 & 63.53 & 63.40 & 57.52 & 58.19 & 40.52 & 37.85 \\ 

\bottomrule
\end{tabular}
\end{table*}

\begin{table*}[!t]\centering
\caption{38 testing 38 20}\label{tab:38_test_38 }
\scriptsize
\begin{tabular}{c|ccccc|ccccc|ccccc}\toprule
&\multicolumn{5}{c|}{Minmax Norm} &\multicolumn{5}{c|}{Standard Norm} &\multicolumn{5}{c}{Robust Norm} \\\cmidrule{2-16}
&3 &5 &7 &10 &15 &3 &5 &7 &10 &15 &3 &5 &7 &10 &15 \\\midrule
5 x 5 & 62.50 & 50.04 & 54.96 & 56.65 & 32.48 & 69.08 & 58.71 & 53.45 & 69.85 & 68.74 & 67.76 & 64.90 & 49.99 & 49.64 & 38.61 \\ 
7 x 7 & 70.35 & 70.56 & 66.49 & 65.27 & 53.66 & 69.16 & 65.46 & 66.12 & 70.83 & 66.99 & 58.32 & 54.96 & 54.46 & 54.46 & 49.06 \\ 
10 x 10 & 80.90 & 81.22 & 81.35 & 75.40 & 71.38 & 80.48 & 80.51 & 81.43 & 79.48 & 73.95 & 60.67 & 53.93 & 55.83 & 53.24 & 46.92 \\ 
15 x 15 & 
\bf{84.13} & 80.96 & 80.53 & 75.19 & 68.08 & 82.23 & 81.43 & 80.03 & 80.90 & 75.80 & 68.74 & 67.18 & 53.03 & 49.25 & 40.33 \\ 
20 x 20 & 81.30 & 77.52 & 80.11 & 76.96 & 73.05 & 78.74 & 78.44 & 74.77 & 73.60 & 68.16 & 67.63 & 65.38 & 61.12 & 61.28 & 55.75 \\ 
25 x 25 & 82.68 & 81.33 & 79.24 & 79.87 & 75.77 & 77.28 & 77.52 & 73.34 & 69.72 & 66.78 & 73.74 & 72.73 & 71.78 & 70.56 & 64.24 \\ 
\bottomrule
\end{tabular}
\end{table*}

\begin{table*}[!t]\centering
\caption{38 Testing all 5}\label{tab:38_test }
\scriptsize
\begin{tabular}{c|ccc|ccc|ccc}\toprule
&\multicolumn{3}{c|}{Minmax Norm} &\multicolumn{3}{c|}{Standard Norm} &\multicolumn{3}{c}{Robust Norm} \\\cmidrule{2-10}
&3 &5 &7   &3 &5 &7  &3 &5 &7   \\\midrule
5 x 5 & 25.19 & 22.61 & 25.00 & 73.42 & 29.70 & 20.32 & 67.40 & 68.29 & 7.23 \\ 
7 x 7 & 78.34 & 71.53 & 61.50 & 76.02 & \bf{81.04} & 74.74 & 67.25 & 67.25 & 67.53 \\ 
10 x 10 & 80.83 & 75.22 & 61.64 & 79.77 & 77.57 & 64.48 & 67.53 & 68.72 & 68.46 \\ 

\bottomrule
\end{tabular}
\end{table*}

\begin{table*}[!t]\centering
\caption{38 testing all 10}\label{tab:343638_vali }
\scriptsize
\begin{tabular}{c|cccc|cccc|cccc}\toprule
&\multicolumn{4}{c|}{Minmax Norm} &\multicolumn{4}{c|}{Standard Norm} &\multicolumn{4}{c}{Robust Norm} \\\cmidrule{2-13}
&3 &5 &7 &10  &3 &5 &7 &10  &3 &5 &7 &10  \\\midrule
5 x 5 & 78.98 & 78.72 & 23.40 & 27.44 & 69.50 & 74.98 & 74.10 & 30.60 & 67.37 & 68.53 & 68.21 & 68.21 \\ 
7 x 7 & 75.70 & 77.22 & 77.30 & 77.13 & 73.86 & 76.08 & 78.90 & 77.92 & 66.99 & 67.01 & 66.99 & 66.98 \\ 
10 x 10 & 80.69 & 79.93 & 79.01 & 73.65 & 75.67 & 76.09 & 74.74 & 73.62 & 67.14 & 67.14 & 66.89 & 68.24 \\ 
15 x 15 & \bf{82.99} & 81.74 & 80.22 & 75.44 & 75.20 & 76.88 & 74.49 & 75.44 & 52.34 & 68.45 & 67.03 & 66.83 \\ 

\bottomrule
\end{tabular}
\end{table*}

\begin{table*}[!t]\centering
\caption{38 testing all 20}\label{tab:38_test_38 }
\scriptsize
\begin{tabular}{c|ccccc|ccccc|ccccc}\toprule
&\multicolumn{5}{c|}{Minmax Norm} &\multicolumn{5}{c|}{Standard Norm} &\multicolumn{5}{c}{Robust Norm} \\\cmidrule{2-16}
&3 &5 &7 &10 &15 &3 &5 &7 &10 &15 &3 &5 &7 &10 &15 \\\midrule
5 x 5 & 74.46 & 73.82 & 73.66 & 70.95 & 23.04 & 79.94 & 73.71 & 73.84 & 76.85 & 79.59 & 68.53 & 68.39 & 68.39 & 68.21 & 7.23 \\ 
7 x 7 & 81.57 & 81.52 & 81.31 & 79.48 & 72.59 & 77.98 & 70.37 & 74.94 & 80.56 & 82.17 & 67.06 & 67.43 & 66.99 & 66.99 & 67.00 \\ 
10 x 10 & 82.16 & 80.59 & 81.41 & 78.45 & 79.78 & 79.11 & 77.27 & 78.98 & 79.87 & 78.43 & 68.61 & 68.56 & 68.52 & 68.28 & 68.28 \\ 
15 x 15 & 80.91 & 80.89 & 81.55 & 81.40 & 79.09 & 79.26 & 77.88 & 78.58 & 80.04 & 78.79 & 68.41 & 68.31 & 68.27 & 68.19 & 67.13 \\ 
20 x 20 & 81.18 & 80.44 & 81.17 & 81.12 & 80.19 & 80.53 & 80.10 & 80.77 & 81.26 & 78.19 & 14.95 & 68.07 & 68.22 & 29.04 & 66.96 \\ 
25 x 25 & 81.91 & 82.47 & 82.31 & \bf{82.49} & 81.40 & 77.10 & 75.75 & 75.39 & 73.82 & 72.91 & 68.70 & 68.49 & 68.41 & 68.59 & 68.39 \\ 
\bottomrule
\end{tabular}
\end{table*}

\begin{table*}[!t]\centering
\caption{34+36+38 Validation 5}\label{tab:343638_vali }
\scriptsize
\begin{tabular}{c|ccc|ccc|ccc}\toprule
&\multicolumn{3}{c|}{Minmax Norm} &\multicolumn{3}{c|}{Standard Norm} &\multicolumn{3}{c}{Robust Norm} \\\cmidrule{2-10}
&3 &5 &7   &3 &5 &7  &3 &5 &7   \\\midrule
5 x 5 & 16.67 & 20.00 & 13.33 & 60.00 & 33.33 & 40.00 & 3.33 & 3.33 & 6.67 \\ 
7 x 7 & 23.33 & 16.67 & 10.00 & 50.00 & 53.33 & 53.33 & 23.33 & 10.00 & 20.00 \\ 
10 x 10 & 30.00 & 33.33 & 16.67 & \bf{56.67} & \bf{56.67} & 43.33 & 33.33 & 23.33 & 23.33 \\ 

\bottomrule
\end{tabular}
\end{table*}

\begin{table*}[!t]\centering
\caption{34+36+38 Validation 10}\label{tab:343638_vali }
\scriptsize
\begin{tabular}{c|cccc|cccc|cccc}\toprule
&\multicolumn{4}{c|}{Minmax Norm} &\multicolumn{4}{c|}{Standard Norm} &\multicolumn{4}{c}{Robust Norm} \\\cmidrule{2-13}
&3 &5 &7 &10  &3 &5 &7 &10  &3 &5 &7 &10  \\\midrule
5 x 5 & 20.00 & 16.67 & 20.00 & 18.33 & 50.00 & 43.33 & 38.33 & 23.33 & 15.00 & 15.00 & 15.00 & 13.33 \\ 
7 x 7 & 45.00 & 40.00 & 33.33 & 31.67 & 43.33 & 43.33 & 40.00 & 45.00 & 25.00 & 20.00 & 20.00 & 18.33 \\ 
10 x 10 & 45.00 & 40.00 & 28.33 & 28.33 & 51.67 & 55.00 & 56.67 & 50.00 & 26.67 & 30.00 & 28.33 & 30.00 \\ 
15 x 15 & 58.33 & 60.00 & 50.00 & 56.67 & 51.67 & 55.00 & 53.33 & \bf{65.00} & 45.00 & 53.33 & 45.00 & 33.33 \\ 

\bottomrule
\end{tabular}
\end{table*}

\begin{table*}[!t]\centering
\caption{34+36+38 Validation 20}\label{tab:343638_vali }
\scriptsize
\begin{tabular}{c|ccccc|ccccc|ccccc}\toprule
&\multicolumn{5}{c|}{Minmax Norm} &\multicolumn{5}{c|}{Standard Norm} &\multicolumn{5}{c}{Robust Norm} \\\cmidrule{2-16}
&3 &5 &7 &10 &15 &3 &5 &7 &10 &15 &3 &5 &7 &10 &15 \\\midrule
5 x 5 & 31.67 & 28.33 & 20.83 & 17.50 & 13.33 & 53.33 & 50.00 & 44.17 & 45.83 & 48.33 & 21.67 & 21.67 & 19.17 & 19.17 & 16.67 \\ 
7 x 7 & 45.00 & 45.00 & 31.67 & 43.33 & 37.50 & 38.33 & 45.83 & 49.17 & 50.00 & 51.67 & 27.50 & 25.83 & 26.67 & 16.67 & 15.00 \\ 
10 x 10 & 56.67 & 50.83 & 39.17 & 40.83 & 32.50 & 71.67 & 75.83 & 64.17 & 58.33 & 55.83 & 25.83 & 30.83 & 30.83 & 24.17 & 26.67 \\ 
15 x 15 & 67.50 & 67.50 & 68.33 & 68.33 & 65.00 & 60.83 & 63.33 & 56.67 & 58.33 & 50.83 & 57.50 & 60.00 & 60.83 & 53.33 & 44.17 \\ 
20 x 20 & 55.00 & 60.00 & 56.67 & 56.67 & 48.33 & 76.67 & 73.33 & 77.50 & 72.50 & 68.33 & 55.83 & 62.50 & 61.67 & 52.50 & 50.00 \\ 
25 x 25 & \bf{82.50} & 80.00 & 78.33 & 72.50 & 50.83 & 65.00 & 68.33 & 65.00 & 64.17 & 64.17 & 54.17 & 60.00 & 61.67 & 55.83 & 46.67 \\ 

\bottomrule
\end{tabular}
\end{table*}

\begin{table*}[!t]\centering
\caption{34+36+38 Validation 30}\label{tab:343638_vali }
\scriptsize
\begin{tabular}{c|ccccc|ccccc|ccccc}\toprule
&\multicolumn{5}{c|}{Minmax Norm} &\multicolumn{5}{c|}{Standard Norm} &\multicolumn{5}{c}{Robust Norm} \\\cmidrule{2-16}
&3 &5 &7 &10 &15 &3 &5 &7 &10 &15 &3 &5 &7 &10 &15 \\\midrule
5 x 5 & 35.56 & 31.67 & 33.89 & 32.78 & 35.00 & 58.33 & 60.00 & 57.22 & 43.89 & 45.56 & 13.33 & 16.11 & 11.67 & 12.22 & 13.33 \\ 
7 x 7 & 40.56 & 40.00 & 35.00 & 32.22 & 22.22 & 45.00 & 45.56 & 48.89 & 44.44 & 33.33 & 29.44 & 25.56 & 25.56 & 26.67 & 25.56 \\ 
10 x 10 & 54.44 & 53.89 & 50.56 & 58.33 & 56.67 & 60.00 & 60.00 & 59.44 & 62.78 & 60.00 & 45.00 & 46.11 & 55.56 & 53.33 & 46.67 \\ 
15 x 15 & 56.67 & 58.33 & 61.11 & 61.11 & 50.56 & 63.33 & 61.67 & 61.67 & 63.33 & 58.33 & 59.44 & 56.67 & 53.89 & 56.11 & 41.67 \\ 
20 x 20 & 62.22 & 63.89 & 65.00 & 65.56 & 65.56 & 72.22 & 75.00 & 74.44 & 72.22 & 67.78 & 63.33 & 60.00 & 60.56 & 65.00 & 54.44 \\ 
25 x 25 & 72.78 & 77.78 & \bf{78.33} & 75.56 & 72.78 & 71.67 & 68.89 & 72.22 & 72.78 & 75.00 & 53.89 & 57.78 & 53.89 & 53.89 & 52.22 \\ 

\bottomrule
\end{tabular}
\end{table*}

\begin{table*}[!t]\centering
\caption{34+36+38 Validation 40}\label{tab:343638_vali }
\scriptsize
\begin{tabular}{c|ccccc|ccccc|ccccc}\toprule
&\multicolumn{5}{c|}{Minmax Norm} &\multicolumn{5}{c|}{Standard Norm} &\multicolumn{5}{c}{Robust Norm} \\\cmidrule{2-16}
&3 &5 &7 &10 &15 &3 &5 &7 &10 &15 &3 &5 &7 &10 &15 \\\midrule
5 x 5 & 37.08 & 36.67 & 36.25 & 35.83 & 38.33 & 43.33 & 51.67 & 49.17 & 48.33 & 39.58 & 15.42 & 15.42 & 15.00 & 14.58 & 12.08 \\ 
7 x 7 & 37.92 & 39.58 & 38.75 & 36.67 & 39.58 & 43.75 & 40.83 & 38.75 & 41.25 & 44.17 & 38.75 & 38.33 & 37.08 & 38.33 & 25.00 \\ 
10 x 10 & 55.83 & 59.17 & 47.50 & 53.75 & 52.50 & 54.58 & 58.75 & 57.50 & 48.75 & 47.08 & 42.50 & 46.25 & 46.25 & 55.83 & 49.58 \\ 
15 x 15 & 60.42 & 64.17 & 64.17 & 57.92 & 62.08 & 67.08 & 53.33 & 60.00 & 62.50 & 61.25 & 51.25 & 48.33 & 47.08 & 47.08 & 43.33 \\ 
20 x 20 & 61.67 & 59.17 & 69.17 & 60.83 & 61.25 & \bf{75.83} & 72.50 & \bf{75.83} & \bf{75.83} & 68.75 & 54.58 & 59.17 & 60.83 & 61.25 & 60.83 \\ 
25 x 25 & 66.67 & 75.42 & \bf{75.83} & 73.75 & 73.33 & 69.17 & 72.50 & 68.33 & 64.58 & 68.33 & 64.58 & 62.92 & 59.17 & 58.75 & 58.75 \\ 

\bottomrule
\end{tabular}
\end{table*}

\begin{table*}[!t]\centering
\caption{34+36+38 test 343638 5}\label{tab:343638_test }
\scriptsize
\begin{tabular}{c|ccc|ccc|ccc}\toprule
&\multicolumn{3}{c|}{Minmax Norm} &\multicolumn{3}{c|}{Standard Norm} &\multicolumn{3}{c}{Robust Norm} \\\cmidrule{2-10}
&3 &5 &7   &3 &5 &7  &3 &5 &7   \\\midrule

5 x 5 & 41.54 & 39.00 & 38.18 & 65.94 & 42.18 & 53.05 & 30.88 & 30.75 & 29.75 \\ 
7 x 7 & 51.87 & 44.82 & 36.69 & 69.25 & 62.63 & 60.95 & 64.29 & 47.70 & 44.71 \\ 
10 x 10 & 46.94 & 53.17 & 41.80 & \bf{72.32} & 69.50 & 52.41 & 62.28 & 56.03 & 60.74 \\ 
\bottomrule
\end{tabular}
\end{table*}

\begin{table*}[!t]\centering
\caption{34+36+38 test 343638 10}\label{tab:343638_test }
\scriptsize
\begin{tabular}{c|cccc|cccc|cccc}\toprule
&\multicolumn{4}{c|}{Minmax Norm} &\multicolumn{4}{c|}{Standard Norm} &\multicolumn{4}{c}{Robust Norm} \\\cmidrule{2-13}
&3 &5 &7 &10  &3 &5 &7 &10  &3 &5 &7 &10  \\\midrule

5 x 5 & 32.19 & 18.76 & 42.55 & 41.64 & 74.78 & 69.26 & 51.00 & 47.99 & 39.64 & 39.64 & 40.09 & 39.78 \\ 
7 x 7 & 74.09 & 59.02 & 44.48 & 47.86 & 64.52 & 75.33 & 68.67 & 73.73 & 61.56 & 58.61 & 67.69 & 66.40 \\ 
10 x 10 & 63.80 & 52.81 & 51.92 & 49.67 & 68.37 & 66.75 & 66.89 & 64.54 & 58.33 & 59.69 & 64.09 & 65.06 \\ 
15 x 15 & \bf{76.44} & 76.00 & 70.65 & 72.81 & 67.15 & 65.25 & 66.34 & 67.05 & 53.49 & 60.45 & 54.91 & 48.99 \\ 
\bottomrule
\end{tabular}
\end{table*}

\begin{table*}[!t]\centering
\caption{34+36+38 test 343638 20}\label{tab:343638_test }
\scriptsize
\begin{tabular}{c|ccccc|ccccc|ccccc}\toprule
&\multicolumn{5}{c|}{Minmax Norm} &\multicolumn{5}{c|}{Standard Norm} &\multicolumn{5}{c}{Robust Norm} \\\cmidrule{2-16}
&3 &5 &7 &10 &15 &3 &5 &7 &10 &15 &3 &5 &7 &10 &15 \\\midrule
5 x 5 & 45.41 & 47.34 & 38.01 & 38.09 & 34.77 & \bf{85.12} & 71.24 & 68.00 & 59.19 & 67.79 & 45.29 & 45.29 & 44.06 & 44.06 & 39.15 \\ 
7 x 7 & 64.81 & 64.18 & 51.06 & 49.90 & 47.70 & 68.83 & 68.68 & 70.42 & 71.98 & 65.50 & 67.50 & 63.58 & 61.25 & 52.26 & 47.49 \\ 
10 x 10 & 79.71 & 70.06 & 57.51 & 51.65 & 52.98 & 70.89 & 71.22 & 70.45 & 66.77 & 60.65 & 62.60 & 66.34 & 58.80 & 41.62 & 36.98 \\ 
15 x 15 & 82.73 & 81.07 & 78.09 & 77.86 & 72.52 & 69.74 & 68.23 & 64.11 & 65.19 & 62.10 & 73.50 & 69.79 & 71.83 & 64.74 & 55.20 \\ 
20 x 20 & 83.22 & 78.04 & 75.29 & 73.82 & 68.93 & 75.09 & 68.32 & 67.29 & 65.97 & 61.00 & 72.92 & 72.18 & 71.59 & 68.13 & 64.91 \\ 
25 x 25 & 79.57 & 79.24 & 79.51 & 74.97 & 63.37 & 75.15 & 75.75 & 71.38 & 72.11 & 61.13 & 73.93 & 73.55 & 72.46 & 71.35 & 67.42 \\ 
\bottomrule
\end{tabular}
\end{table*}

\begin{table*}[!t]\centering
\caption{34+36+38 test 343638 30}\label{tab:343638_test }
\scriptsize
\begin{tabular}{c|ccccc|ccccc|ccccc}\toprule
&\multicolumn{5}{c|}{Minmax Norm} &\multicolumn{5}{c|}{Standard Norm} &\multicolumn{5}{c}{Robust Norm} \\\cmidrule{2-16}
&3 &5 &7 &10 &15 &3 &5 &7 &10 &15 &3 &5 &7 &10 &15 \\\midrule
5 x 5 & 53.29 & 53.18 & 46.42 & 41.62 & 52.38 & 80.87 & 81.77 & 80.51 & 70.00 & 75.03 & 42.30 & 38.41 & 40.24 & 39.54 & 41.78 \\ 
7 x 7 & 67.80 & 69.13 & 54.35 & 54.36 & 46.93 & 70.55 & 70.53 & 67.05 & 63.28 & 62.00 & 67.49 & 68.83 & 68.83 & 67.18 & 66.97 \\ 
10 x 10 & 73.07 & 73.59 & 67.91 & 74.44 & 70.71 & 75.21 & 71.86 & 71.11 & 72.58 & 67.20 & 74.72 & 74.30 & 72.58 & 62.72 & 73.67 \\ 
15 x 15 & 82.54 & 80.87 & 76.85 & 76.47 & 72.61 & 76.70 & 75.01 & 75.23 & 69.52 & 67.19 & 78.21 & 75.41 & 74.28 & 72.59 & 65.51 \\ 
20 x 20 & 84.25 & 80.61 & 78.76 & 80.19 & 77.58 & 83.26 & 79.05 & 74.70 & 72.90 & 61.76 & 77.64 & 71.64 & 77.48 & 78.34 & 72.89 \\ 
25 x 25 & \bf{85.52} & 82.32 & 79.72 & 78.40 & 76.22 & 82.37 & 83.63 & 80.89 & 78.31 & - & 75.60 & 75.31 & 73.65 & 75.22 & - \\ 
\bottomrule
\end{tabular}
\end{table*}

\begin{table*}[!t]\centering
\caption{34+36+38 test 343638 40}\label{tab:343638_test }
\scriptsize
\begin{tabular}{c|ccccc|ccccc|ccccc}\toprule
&\multicolumn{5}{c|}{Minmax Norm} &\multicolumn{5}{c|}{Standard Norm} &\multicolumn{5}{c}{Robust Norm} \\\cmidrule{2-16}
&3 &5 &7 &10 &15 &3 &5 &7 &10 &15 &3 &5 &7 &10 &15 \\\midrule
5 x 5 & 57.16 & 51.40 & 42.40 & 42.58 & 46.02 & 73.44 & 77.30 & 76.36 & 74.44 & 62.65 & 38.28 & 38.28 & 36.04 & 40.17 & 37.51 \\ 
7 x 7 & 67.72 & 68.10 & 66.26 & 61.81 & 66.67 & 77.40 & 71.60 & 66.50 & 66.86 & 66.74 & 65.44 & 63.31 & 62.34 & 62.61 & 62.54 \\ 
10 x 10 & 80.23 & 81.78 & 71.00 & 69.74 & 68.84 & 78.54 & 75.79 & 74.19 & 68.07 & 67.66 & 66.04 & 69.28 & 69.28 & 71.19 & 65.20 \\ 
15 x 15 & 81.82 & 82.42 & 78.93 & 78.79 & 74.88 & 71.08 & 70.17 & 69.01 & 64.55 & 65.77 & 72.61 & 70.76 & 69.47 & 70.23 & 63.91 \\ 
20 x 20 & 82.02 & 78.42 & 79.01 & 78.21 & 75.09 & 81.82 & 78.22 & 78.71 & 77.73 & 69.64 & 75.75 & 73.48 & 71.79 & 68.91 & 66.58 \\ 
25 x 25 & 83.93 & \bf{84.68} & 80.14 & 79.29 & 74.84 & 80.62 & 80.39 & 75.58 & 76.62 & 70.39 & 73.89 & 73.60 & 70.74 & 68.04 & 70.00 \\ 

\bottomrule
\end{tabular}
\end{table*}

\begin{table*}[!t]\centering
\caption{34+36+38 test all 5}\label{tab:343638_vali }
\scriptsize
\begin{tabular}{c|ccc|ccc|ccc}\toprule
&\multicolumn{3}{c|}{Minmax Norm} &\multicolumn{3}{c|}{Standard Norm} &\multicolumn{3}{c}{Robust Norm} \\\cmidrule{2-10}
&3 &5 &7   &3 &5 &7  &3 &5 &7   \\\midrule
5 x 5 & 39.16 & 38.00 & 37.53 & 60.90 & 39.50 & 48.04 & 35.98 & 35.87 & 35.18 \\ 
7 x 7 & 46.40 & 40.35 & 35.26 & 69.03 & 63.26 & 62.95 & 60.62 & 45.85 & 48.52 \\ 
10 x 10 & 45.20 & 51.29 & 40.37 & \bf{70.34} & 69.73 & 48.90 & 65.17 & 57.74 & 65.05 \\ 

\bottomrule
\end{tabular}
\end{table*}

\begin{table*}[!t]\centering
\caption{34+36+38 test all 10}\label{tab:343638_vali }
\scriptsize
\begin{tabular}{c|cccc|cccc|cccc}\toprule
&\multicolumn{4}{c|}{Minmax Norm} &\multicolumn{4}{c|}{Standard Norm} &\multicolumn{4}{c}{Robust Norm} \\\cmidrule{2-13}
&3 &5 &7 &10  &3 &5 &7 &10  &3 &5 &7 &10  \\\midrule
5 x 5 & 29.63 & 18.00 & 40.79 & 40.00 & 67.75 & 66.57 & 48.43 & 47.38 & 42.86 & 42.86 & 44.74 & 44.47 \\ 
7 x 7 & 66.64 & 55.92 & 43.64 & 46.84 & 64.97 & \bf{75.11} & 70.90 & 73.03 & 56.34 & 55.53 & 63.38 & 63.42 \\ 
10 x 10 & 60.08 & 50.58 & 51.74 & 49.94 & 64.66 & 63.00 & 63.02 & 62.08 & 58.50 & 60.98 & 60.13 & 67.15 \\ 
15 x 15 & 70.12 & 69.03 & 62.70 & 66.16 & 61.63 & 60.87 & 61.43 & 61.50 & 52.91 & 57.60 & 54.28 & 48.52 \\ 

\bottomrule
\end{tabular}
\end{table*}

\begin{table*}[!t]\centering
\caption{34+36+38 test all 20}\label{tab:343638_test }
\scriptsize
\begin{tabular}{c|ccccc|ccccc|ccccc}\toprule
&\multicolumn{5}{c|}{Minmax Norm} &\multicolumn{5}{c|}{Standard Norm} &\multicolumn{5}{c}{Robust Norm} \\\cmidrule{2-16}
&3 &5 &7 &10 &15 &3 &5 &7 &10 &15 &3 &5 &7 &10 &15 \\\midrule
5 x 5 & 41.64 & 44.31 & 35.04 & 34.94 & 32.31 & \bf{79.38} & 66.07 & 63.19 & 55.52 & 63.30 & 47.96 & 47.96 & 46.86 & 46.86 & 42.84 \\ 
7 x 7 & 59.58 & 57.90 & 45.62 & 45.15 & 44.51 & 67.24 & 67.91 & 69.22 & 71.24 & 64.83 & 64.71 & 61.46 & 58.99 & 50.66 & 47.01 \\ 
10 x 10 & 71.74 & 62.92 & 52.46 & 48.63 & 52.12 & 64.83 & 67.08 & 67.51 & 63.28 & 56.96 & 62.32 & 64.79 & 56.08 & 41.01 & 33.45 \\ 
15 x 15 & 75.22 & 73.26 & 70.37 & 70.47 & 64.68 & 69.84 & 67.03 & 62.27 & 61.24 & 57.92 & 70.53 & 67.23 & 68.44 & 61.99 & 54.19 \\ 
20 x 20 & 78.84 & 72.84 & 67.94 & 68.39 & 62.13 & 72.45 & 66.94 & 64.79 & 63.90 & 59.05 & 67.90 & 64.91 & 66.58 & 64.02 & 61.72 \\ 
25 x 25 & 76.12 & 73.90 & 73.56 & 68.84 & 58.47 & 72.50 & 74.55 & 70.55 & 71.25 & 57.99 & 70.18 & 70.13 & 69.44 & 68.74 & 64.39 \\  

\bottomrule
\end{tabular}
\end{table*}

\begin{table*}[!t]\centering
\caption{34+36+38 test all 30}\label{tab:343638_vali }
\scriptsize
\begin{tabular}{c|ccccc|ccccc|ccccc}\toprule
&\multicolumn{5}{c|}{Minmax Norm} &\multicolumn{5}{c|}{Standard Norm} &\multicolumn{5}{c}{Robust Norm} \\\cmidrule{2-16}
&3 &5 &7 &10 &15 &3 &5 &7 &10 &15 &3 &5 &7 &10 &15 \\\midrule
5 x 5 & 45.56 & 50.22 & 42.85 & 39.41 & 47.96 & 77.63 & 75.88 & 74.34 & 64.05 & 70.68 & 46.02 & 42.44 & 44.73 & 42.78 & 45.41 \\ 
7 x 7 & 63.64 & 66.10 & 49.11 & 48.94 & 42.03 & 71.24 & 71.52 & 67.33 & 60.88 & 59.88 & 67.34 & 68.38 & 68.38 & 66.50 & 64.08 \\ 
10 x 10 & 69.00 & 68.71 & 64.28 & 70.78 & 66.17 & 74.06 & 69.40 & 68.68 & 68.12 & 62.65 & 70.51 & 69.80 & 67.20 & 58.11 & 69.05 \\ 
15 x 15 & 75.11 & 75.00 & 69.27 & 68.43 & 63.97 & 74.74 & 74.12 & 73.50 & 67.76 & 64.61 & 73.46 & 71.06 & 69.70 & 68.78 & 63.45 \\ 
20 x 20 & 77.09 & 74.46 & 73.79 & 73.83 & 71.21 & 80.37 & 78.37 & 73.05 & 70.67 & 59.90 & 70.41 & 64.95 & 70.54 & 70.76 & 66.12 \\ 
25 x 25 & 78.43 & 75.93 & 73.11 & 72.78 & 71.06 & 80.85 & \bf{82.44} & 79.63 & 75.96 & 69.18 & 73.32 & 73.82 & 71.94 & 72.62 & 68.58 \\ 
\bottomrule
\end{tabular}
\end{table*}

\begin{table*}[!t]\centering
\caption{34+36+38 test all 40}\label{tab:343638_vali }
\scriptsize
\begin{tabular}{c|ccccc|ccccc|ccccc}\toprule
&\multicolumn{5}{c|}{Minmax Norm} &\multicolumn{5}{c|}{Standard Norm} &\multicolumn{5}{c}{Robust Norm} \\\cmidrule{2-16}
&3 &5 &7 &10 &15 &3 &5 &7 &10 &15 &3 &5 &7 &10 &15 \\\midrule
5 x 5 & 51.77 & 44.43 & 38.07 & 38.29 & 42.72 & 72.58 & 74.95 & 74.02 & 71.01 & 57.53 & 42.32 & 42.32 & 39.69 & 43.47 & 40.33 \\ 
7 x 7 & 58.65 & 58.76 & 57.88 & 54.29 & 59.99 & 75.33 & 70.48 & 67.49 & 67.58 & 66.83 & 61.63 & 59.75 & 58.70 & 58.97 & 60.47 \\ 
10 x 10 & 73.19 & 73.84 & 63.91 & 63.48 & 63.53 & 76.85 & 71.53 & 70.52 & 66.47 & 64.18 & 61.38 & 65.61 & 65.61 & 71.06 & 66.66 \\ 
15 x 15 & 73.36 & 74.45 & 70.35 & 70.22 & 67.02 & 68.47 & 65.82 & 63.59 & 60.34 & 60.74 & 69.26 & 65.51 & 64.82 & 67.85 & 61.64 \\ 
20 x 20 & 77.06 & 74.28 & 75.31 & 73.45 & 66.95 & 76.35 & 73.66 & 72.87 & 71.69 & 66.34 & 70.70 & 68.59 & 66.99 & 64.95 & 62.23 \\ 
25 x 25 & 76.04 & \bf{77.67} & 74.37 & 73.76 & 69.70 & 76.89 & 76.71 & 72.95 & 73.16 & 66.57 & 70.03 & 71.37 & 67.33 & 65.95 & 66.90 \\ 

\bottomrule
\end{tabular}
\end{table*}
